# Supplementary material for: Wahl's conjecture holds in odd characteristics for symplectic and orthogonal Grassmannians
Source: arXiv:0710.3470 source file (2007-11-07)
Supplement: Supplementary file 1 [file appendix.tex]

\mysection{Appendix}\mylabel{s:appendix}\mylabel{s.appendix}
The purpose of this section is to prove directly (meaning, without
recourse to the second assertion of Theorem~\ref{t:canonical}) 
in an elementary algebraic way that the $B$-canonical elements in
$\End_F(G/B)$,  for~$G$ a classical group,  for which explicit
expressions are written in~\S\ref{s.theorem} are indeed splittings.
We will make use of the local criterion for 
splitting~\cite[Proposition~6]{mr} (see also~\cite[\S1.3]{bk}).     
The linear, symplectic, and orthogonal groups are treated separately.
\mysubsection{The case of $SL_n$}\mylabel{ss:app:linear}
Recall the notion of {`residually normal crossing'} introduced 
in~\cite[Definition~1.6]{lmp} 
(see also~\cite[Exercise~1.3.E.10]{bk}):  a reduced
effective divisor~$D$ on a non-singular variety~$X$ of dimension~$n$
is said to be {\em residually normal crossing\/} at a point~$x$ of~$X$
if there exists a system~$t_1$, \ldots, $t_n$  of local co-ordinates
around~$x$ and functions $f_0$, \ldots, $f_{n-1}$ in $\hat{\sheafo}_{X,x}$
such that 
\begin{itemize}
\item $f_0$ is the local equation for $D$ at $x$, and
\item $f_i\equiv t_{i+1}f_{i+1}\mod{(t_1,\ldots,t_i)}$ for
$i=0,1,\ldots,n-1$,  where we set $f_n=1$.
\end{itemize}
As observed in~\cite[\S1]{lmp},
it follows from the local criterion for splitting 
(see also~\cite[Exercise~1.3.E.11]{bk}) that
if $\sigma$ is a section of the negative canonical bundle~$K^{-1}$ of
a complete non-singular variety such that the divisor defined by its
vanishing is reduced and has residually normal crossing at some point,
then $\sigma^{p-1}$ is a splitting of~$X$.    

We claim that the section $\sectionp\sectionq$ in~\S\ref{ss.sln} of~$K^{-1}$ 
of $SL_n/B$ has residual normal crossing at the identity coset~$eB$.
The image~$U^-$ in $G/B$ under the map $u\mapsto ueB$ is isomorphic 
to~$U^-$ and gives an affine patch of~$G/B$ around~$eB$.  A general
element of~$U^-$ looks like:
\[
\left(\begin{array}{ccccc}
1 \\
&  1 &  & 0 \\
& & \ddots \\
& \star & & 1 \\
& & & & 1\\
\end{array}\right) \]
Clearly $\sectionp$ restricts identically to~$1$ on~$U^-$. 
It suffices therefore to show the following claim: the 
restriction to~$U^-$ of~$\sectionq$
has residually normal crossing at the identity with respect to the `standard' 
co-ordinates~$\star$.

We will write out the proof this claim in the special case~$n=5$ from which
the proof in the general case will be clear.   To write out the proof in
the general case would involve too much notation and thus obfuscate rather
than illuminate the pattern of the proof.

So let $n=5$.   We write a general element of~$U^-$ as:
\[
\left(\begin{array}{ccccc}
1 \\
a &  1  \\
b & c & 1 \\
d & e & f & 1 \\
g & h & i & j & 1\\
\end{array}\right) \]
where $a$, $b$, \ldots, $j$ are affine co-ordinates.   The restriction 
of~$\sectionq$ is given by the product of four determinants:
\[ \sectionq=g\cdot(dh-ge)\cdot(bei-\cdots)\cdot(acfj-\cdots)\]
Take $f_0=\sectionq$, $t_1=g$, 
$f_1=(dh-ge)\cdot(bei-\cdots)\cdot(acfj-\cdots)$, 
$t_2=d$, $f_2=h\cdot(bei-\cdots)\cdot(acfj-\cdots)$ (where now in both
determinants we ignore terms involving~$g$),  $t_3=h$,  
$f_3=(bei-bfh)\cdot(acfj-\cdots)$ (where now in both determinants we
are ignoring terms involving~$g$ or~$d$), $t_4=b$,  
$f_4=ei\cdot(acfj-\cdots)$ (where now in the determinant we are 
ignoring terms involving~$g$, $d$, or~$h$), $t_5=e$,
$f_5=i(acfj-aci-aej)$, $t_6=i$, $f_6=(acfj-aci)$,
$t_7=a$, $f_7=cfj$, $t_8=c$, $f_8=fj$, $t_9=f$, $f_9=j$,
$t_{10}=j$, $f_{10}=1$.
